# Supplementary material for: DIV-FF: Dynamic Image-Video Feature Fields For Environment Understanding in Egocentric Videos
Source: arXiv:2503.08344 source file (2025-03-11)
Supplement: Supplementary file 1 [file supp.tex]

\section{Annotation procedure for the Affordance Segmentation task}

For the evaluation of the Dynamic Object Segmentation task, we reuse the object retrieval task labels from N3F \cite{tschernezki2022neural}. In contrast, we manually annotate the affordance masks in the EPIC-Diff sequences to quantitatively evaluate the Affordance Segmentation task. For each scene, we identified five interactions occurring within the video.
Following the procedure proposed by Nagarajan et. al \cite{nagarajan2019grounded} for interaction hotspots evaluation, we mark 6 points on each image where the interaction could feasibly occur. 
As Figure \ref{fig:supp annot} shows, these annotations are localized on both the relevant parts of the object for the affordance and grounded in real human demonstration.
We then transformed these annotations into a heatmap by centering a Gaussian distribution at each marked point, as shows Figure \ref{fig:supp annot}. 
The ground-truth affordance mask corresponds to the pixels where the heatmap is above 0.5. We show two examples of the binary masks in Figure \ref{fig:supp aff}.
Overall, we collected 872 binary masks between all the sequences. The list of the evaluated affordances is shown in Table \ref{tab:text_queries}. We will release the affordance annotations and the code.

\begin{figure}[ht]
    \centering
    \includegraphics[width=0.99\linewidth]{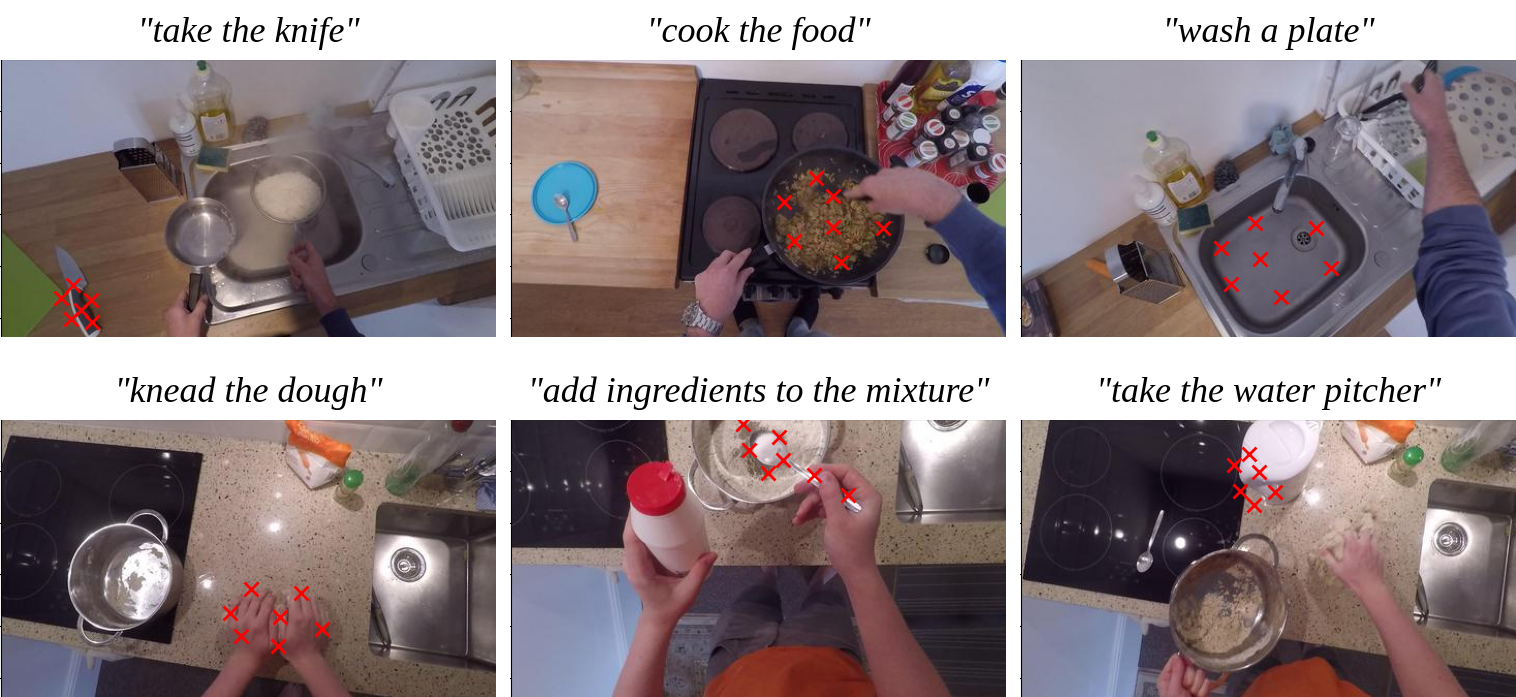}
    \caption{\textbf{Key-points marked for the affordance masks.}}
    \label{fig:supp annot}
\end{figure}

\begin{figure}[ht]
    \centering
    \includegraphics[width=0.99\linewidth]{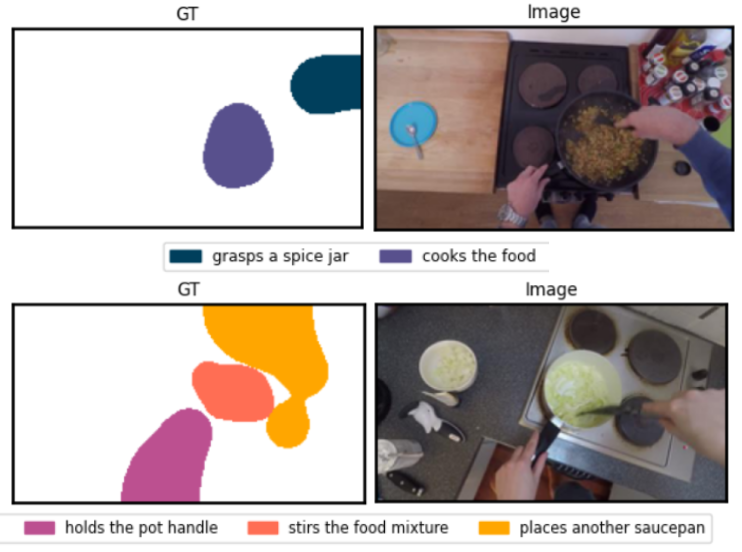}
    \caption{\textbf{Affordance Segmentation ground-truth masks.} From the marked points, we derived a Gaussian heatmap. The evaluation affordance masks corresponds where the heatmap is above 0.5.}
    \label{fig:supp aff}
\end{figure}

\section{Computational details}

\textbf{Training.} 
For geometry reconstruction, we downscale the images from the EPIC Kitchens videos to a resolution of 128 $\times$ 228. 
SAM masks are extracted from higher-resolution images (228 $\times$ 456) to better capture small objects and fine details. Both EgoVideo patches and CLIP tiles are resized to 224 $\times$ 224 prior to feature extraction.
We also train per-scene an auto-encoder to reduce the dimensionality of CLIP embeddings from 512 to 128 following \cite{qin2024langsplat}.

\textbf{Testing.} 
Each scene requires approximately 25MB of disk space, compared to the 17MB needed to store only the geometry reconstruction. 
Since rendering the semantic features is very costly in memory terms, we infer sequentially the persistent, dynamic and actor feature fields during rendering to keep the memory constrains.
Our experiments were conducted on an NVIDIA GeForce RTX 4090, where the rendering time for the LERF baseline is 1.48 seconds. During inference, LERF compares relevancy maps across 30 different scales to select the optimal one.
In contrast, DIV-FF leverages SAM-generated masks to extract CLIP object-aligned features, eliminating the need for multi-scale inference. This reduces DIV-FF's inference time to 0.82 seconds.
It is worth noting that DIV-FF renders both the image and video feature fields, whereas LERF only extracts image-language features.

\begin{table*}[ht]
\resizebox{\textwidth}{!}{%
\begin{tabular}{ccc} %|
\hline
Scene   & Dynamic Objects text queries                                                                           & Affordance Segmentation text queries                                                                                                                                     \\ \hline
P01\_01 & \begin{tabular}[c]{@{}c@{}}green cutting board, blue lid, \\ cheese grater, saucepan, pot\end{tabular} & \begin{tabular}[c]{@{}c@{}}grasp a spice jar, cook the food, \\ wash a plate, cut vegetables, \\ take a knife with right hand\end{tabular}                               \\ \hline
P03\_04 & \begin{tabular}[c]{@{}c@{}}bowl, blue cutting board, \\ knife, pot\end{tabular}                        & \begin{tabular}[c]{@{}c@{}}cut the onion, wash a kitchen utensil, \\ hold the pot handle, stir the food mixture, \\ place another saucepan\end{tabular}                  \\ \hline
P04\_01 & \begin{tabular}[c]{@{}c@{}}white spoon, transparent bottle, \\ white bottle, pan\end{tabular}          & \begin{tabular}[c]{@{}c@{}}turns on the faucet, wash a kitchen utensil, \\ cook the food, open a cabinet\end{tabular}                                                    \\ \hline
P05\_01 & \begin{tabular}[c]{@{}c@{}}cup, electric kettle, \\ banana, milk bottle\end{tabular}                   & \begin{tabular}[c]{@{}c@{}}heat water with the kettle, toast the bread, \\ pour water in the mug, take the bottle milk, \\ heat food in the microwave\end{tabular}       \\ \hline
P06\_03 & \begin{tabular}[c]{@{}c@{}}pot, flour package, \\ jug, orange bag\end{tabular}                         & \begin{tabular}[c]{@{}c@{}}add ingredients to the mixture, wash kitchen utensils, \\ take the water pitcher, open the bag, \\ knead the ingredients\end{tabular}         \\ \hline
P08\_01 & \begin{tabular}[c]{@{}c@{}}frying pan, coffee cup, \\ cutting board, plate\end{tabular}                & \begin{tabular}[c]{@{}c@{}}cook the ingredients, prepare the coffee, \\ cut the ingredients, drink the coffee, \\ spread the mixture on the toast\end{tabular}           \\ \hline
P09\_02 & \begin{tabular}[c]{@{}c@{}}spagueti package, \\ white cutting board, \\ saucepan, plate\end{tabular}   & \begin{tabular}[c]{@{}c@{}}hold the pan, heat water, \\ control the stove, prepare the omelette, \\ wash kitchen utensils\end{tabular}                                   \\ \hline
P13\_03 & \begin{tabular}[c]{@{}c@{}}plate, colander, \\ pasta, scissors\end{tabular}                            & \begin{tabular}[c]{@{}c@{}}drain the pasta, open a drawer, \\ add sauce to the pasta, \\ open the cheese bag, prepare the food\end{tabular}                              \\ \hline
P16\_01 & \begin{tabular}[c]{@{}c@{}}pot, package, \\ knife protector, cutting board\end{tabular}                & \begin{tabular}[c]{@{}c@{}}cut the ingredients, cook the ingredients, \\ wash kitchen utensils, open the package,\\ place a frying pan in an available hob\end{tabular}  \\ \hline
P21\_01 & \begin{tabular}[c]{@{}c@{}}white plate, plastic package, \\ blue plate, paper bag\end{tabular}         & \begin{tabular}[c]{@{}c@{}}open the fridge, soak the tomatoes, \\ manipulate the ingredients, \\ wash kitchen utensils, \\ take a knife with the right hand\end{tabular} \\ \hline
\end{tabular}
}
\caption{\textbf{Text queries used during the Dynamic Objects and Affordance Segmentation evaluation experiments.}}
\label{tab:text_queries}
\end{table*}

\section{Extra qualitative results}

We report extra qualitative results for the image language feature map of DIV-FF in Figure \ref{fig:supp qualit}. 
We first show the PCA feature map of the rendered scene, followed by relevancy maps both for dynamic (\textit{`green cutting board´, `spoon´, `food´...}) and static (\textit{`sink´, `gas cooktop´, `drainer´}) objects. 
We also attach videos depicting the full egocentric video sequence, showcasing views from both the actor's and a static perspective (which is a novel view along all the different time-steps).
Similarly, the video language of DIV-FF is illustrated in Figure~\ref{fig:supp video}, which highlights multiple affordance actions from the same novel viewpoint.

\section{Limitations}

The image-language field of DIV-FF inherits several limitations from SAM, notably in the excessive segmentation of objects that omits some of its parts. This is evident in cases such as the \textit{`cup´} in P04-01, \textit{`plate´} in P13-03 and \textit{`sink´} in P21-01 examples of Figure \ref{fig:supp qualit}. The segmentation produced by SAM either omits some parts of the objects or introduces artifacts such as holes.

\begin{figure*}
    \centering
    \includegraphics[width=0.99\textwidth]{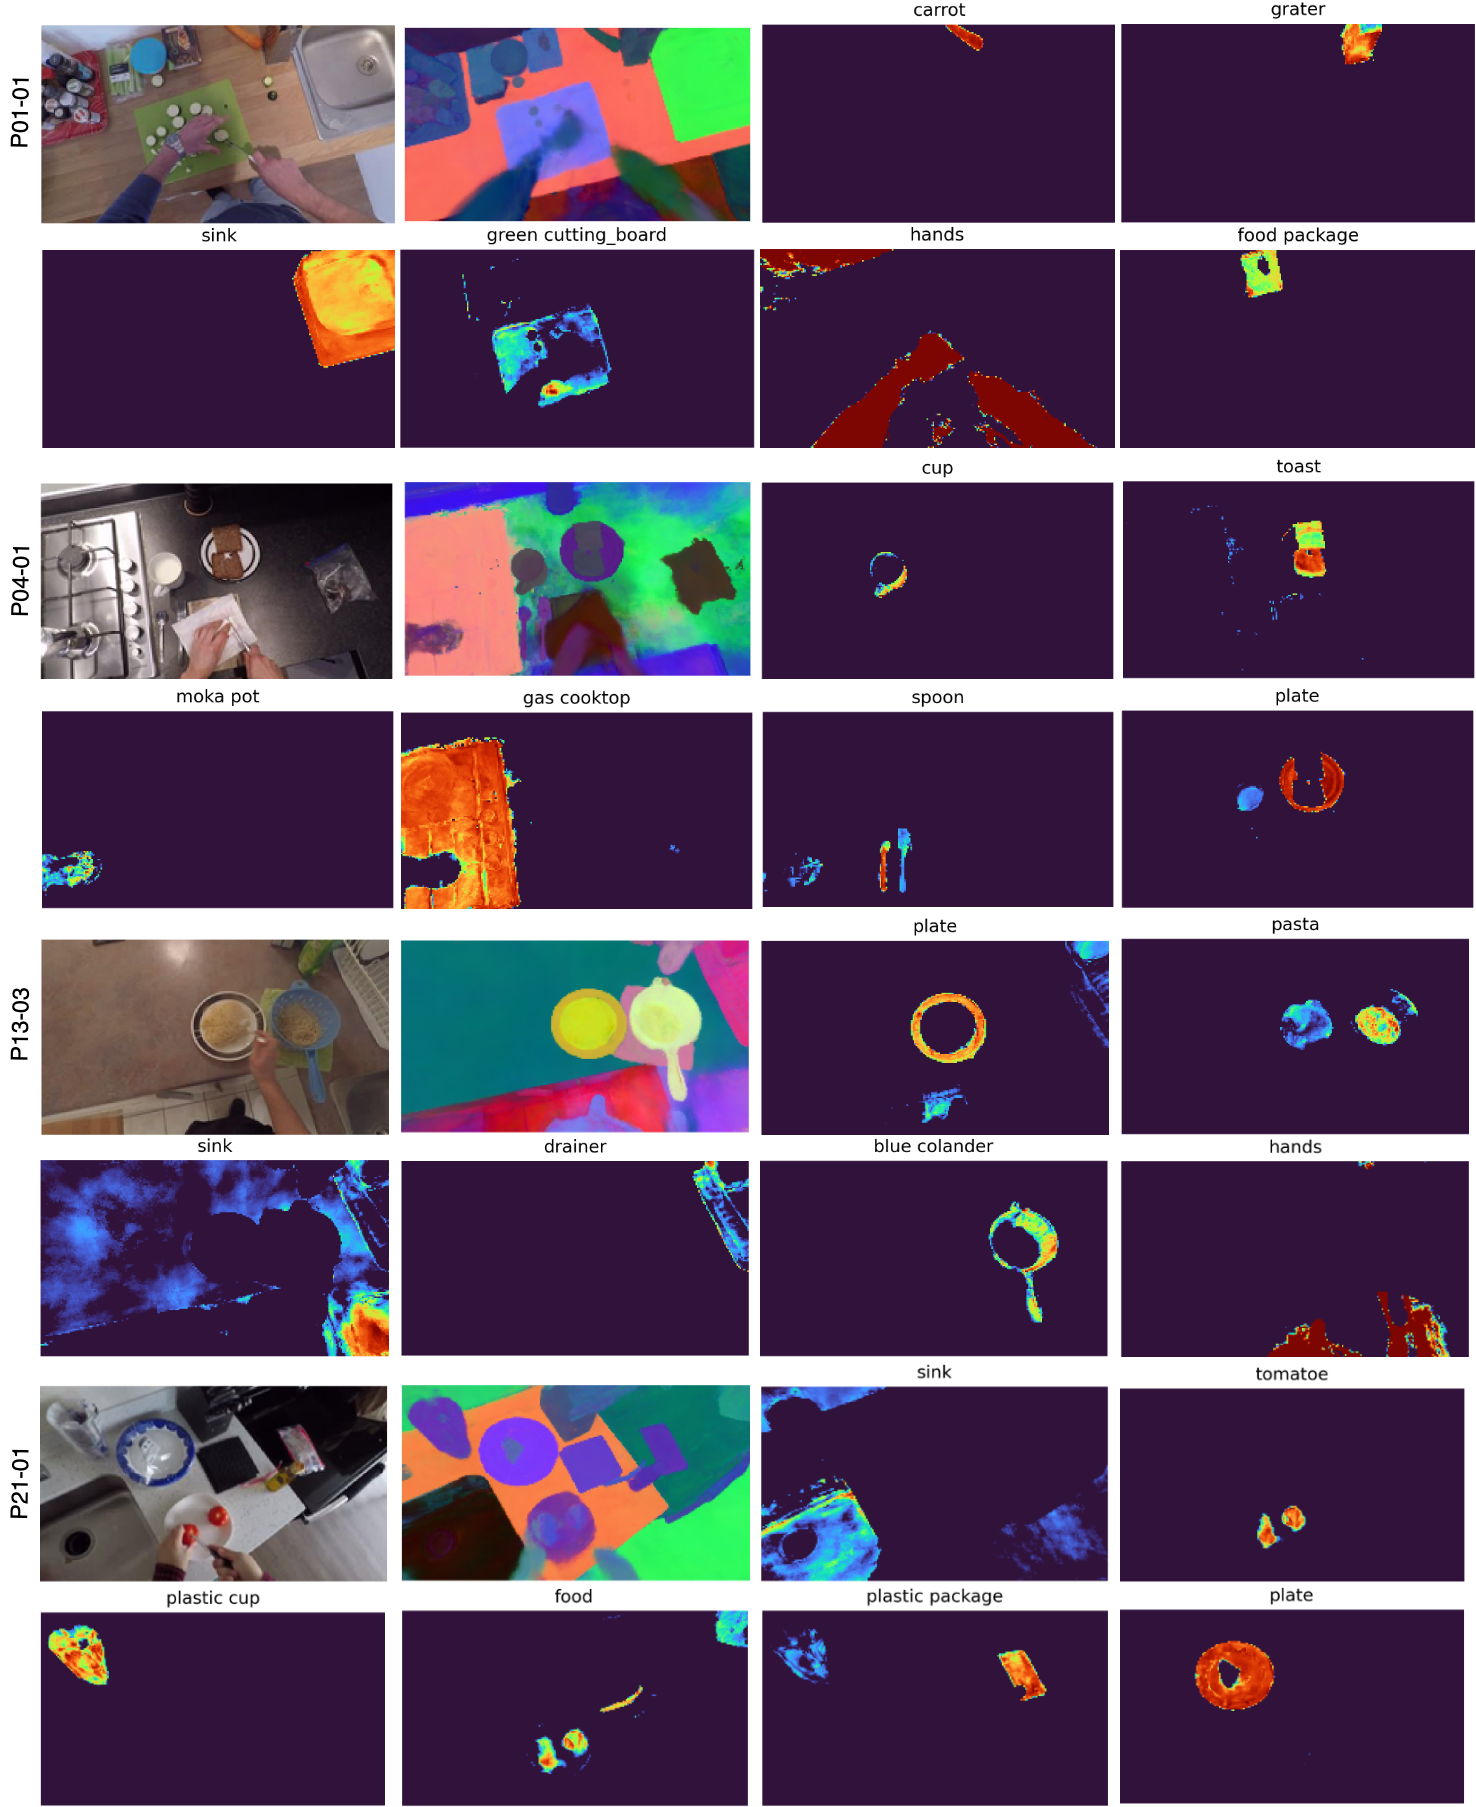}
    \caption{\textbf{Additional results of the DIV-FF Image Language relevancy map in novel views.} We visualize the ground-truth image, the PCA of the image-language features and different relevancy maps for different text queries.}
    \label{fig:supp qualit}
\end{figure*}

\begin{figure*}
    \centering
    \includegraphics[width=0.99\textwidth]{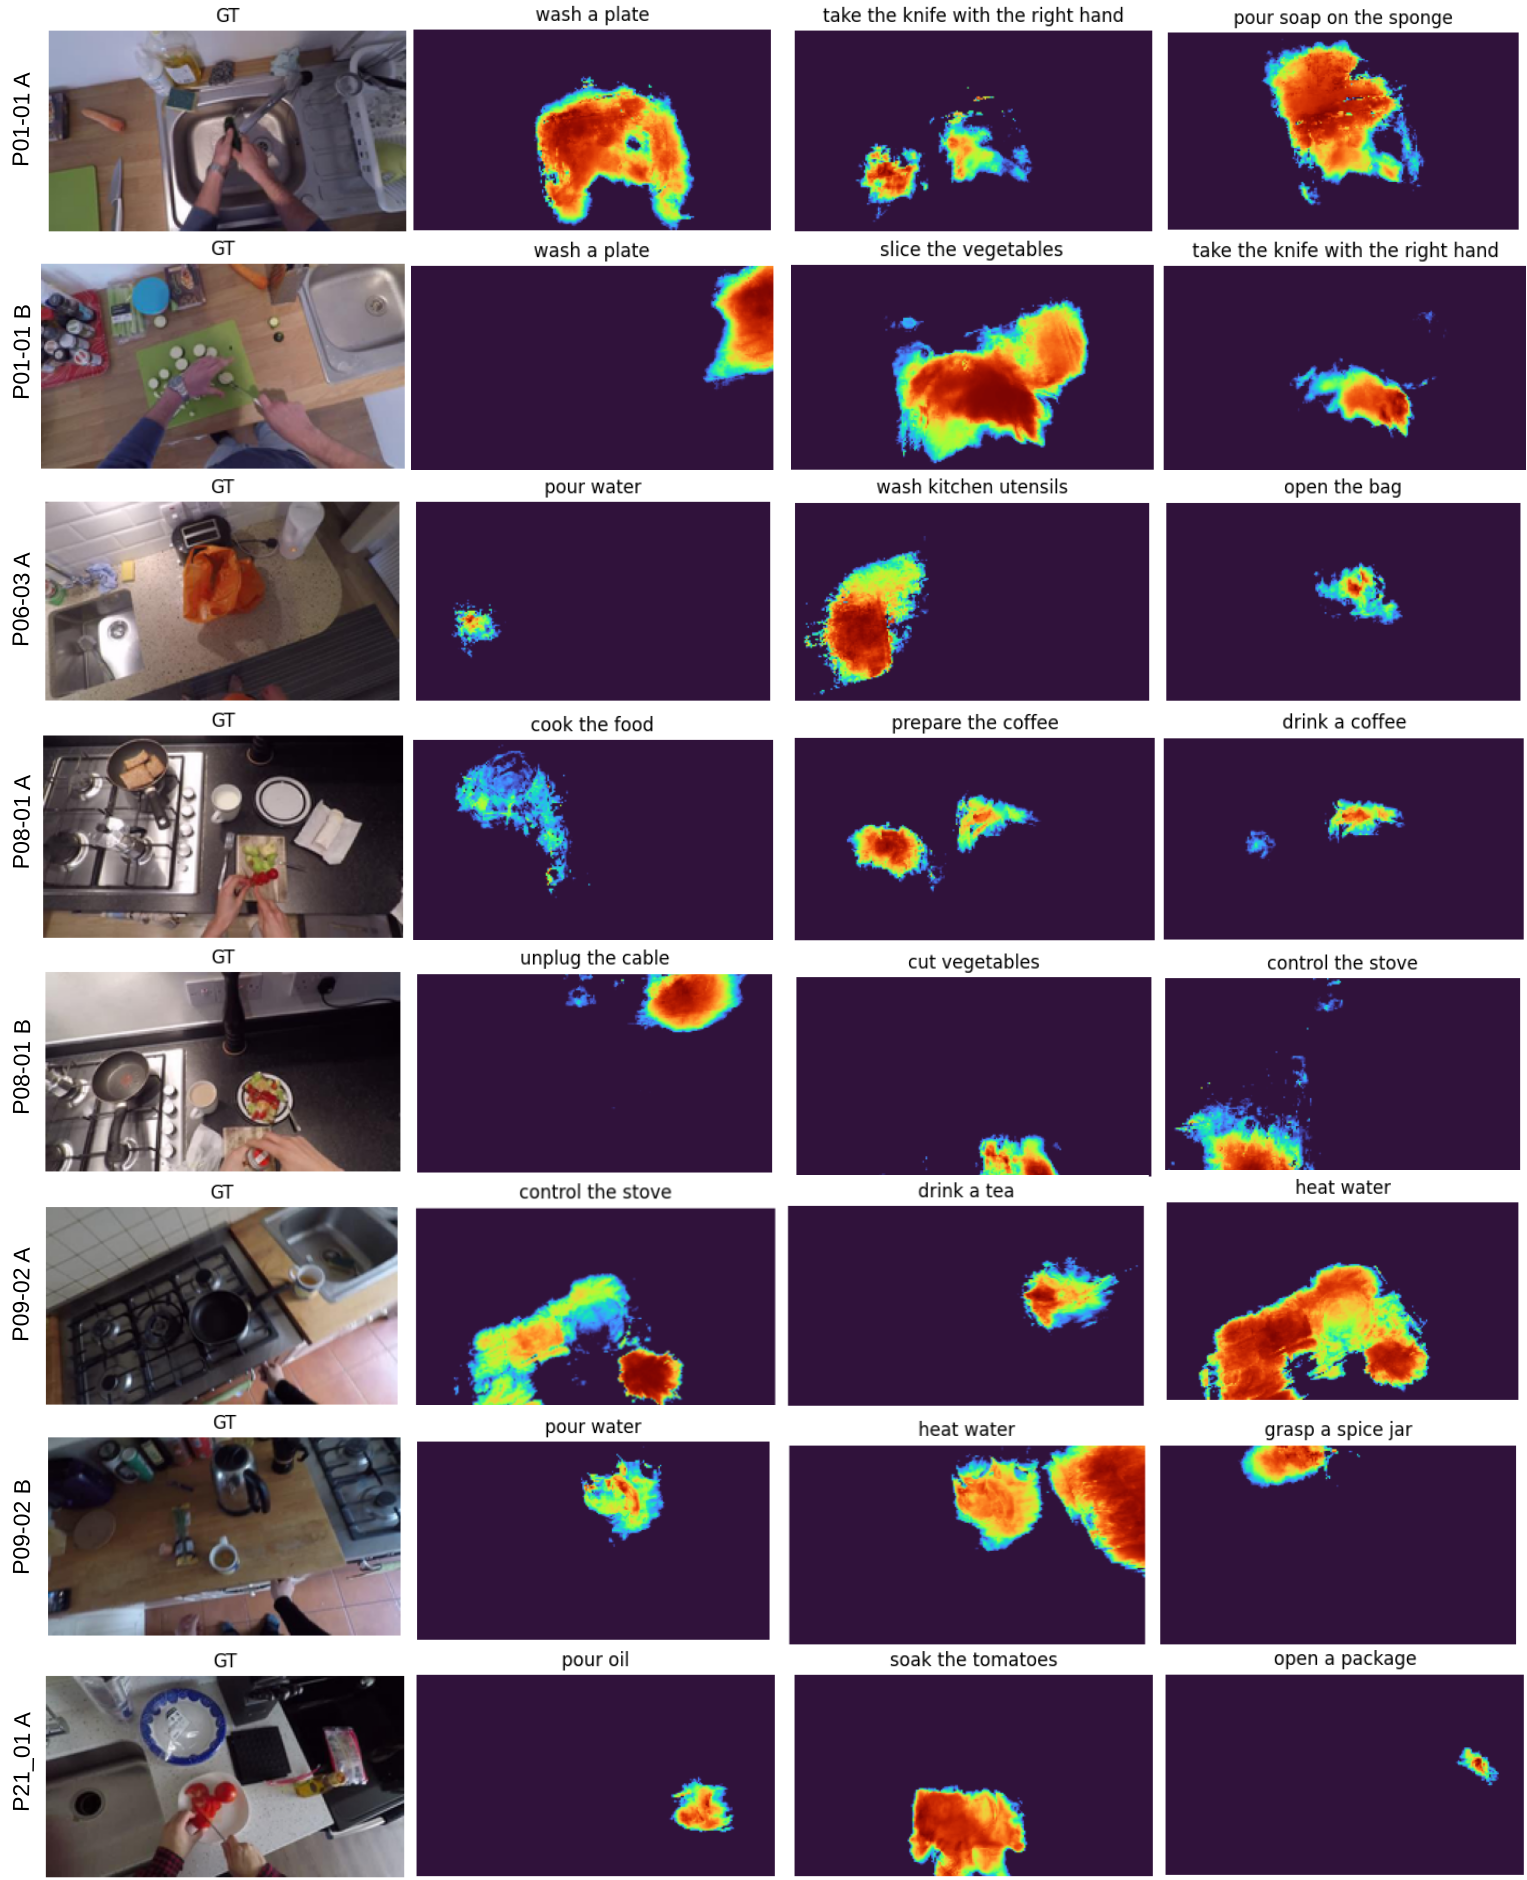}
    \caption{\textbf{Additional results of the DIV-FF Image Language relevancy map in novel views.} We visualize the ground-truth image and three different relevancy maps of the video-language feature field corresponding of affordable interactions.}
    \label{fig:supp video}
\end{figure*}

Another limitation of DIV-FF is the degradation associated to the geometry, specially when rendering the actor's hands (scenes P01-01 and P13-03 in Figure \ref{fig:supp qualit}). The actor’s hands continuous movement and the biased top-view (egocentric) perspective of all the images pose a significant challenge in accurately rendering the hands in novel views, which is later reflected in the relevancy maps for the \textit{`hands´} text query. 

Despite the inclusion of persistent, dynamic and actor streams in DIV-FF to enhance the capture of egocentric video, the rendering quality of objects in contact with the actor, such as the \textit{`green cutting board´} in P01-01 or \textit{`pasta´} in P13-03 in Figure \ref{fig:supp qualit}, is compromised. This degradation is primarily due to frequent occlusions by the actor’s hands, disrupting the continuity of views

The main limitation in the video-language feature field of DIV-FF is the rendering of diffuse relevancy maps, which introduce excessive noise (\textit{`pour soap on the sponge´} in P01-01 A or \textit{`control the stove´} in P09-02 A, both in Figure \ref{fig:supp video}) in some cases.
